# Supplementary material for: Unveiling the Ignorance of MLLMs: Seeing Clearly, Answering Incorrectly
Source: arXiv:2406.10638 source file (2025-03-19)
Supplement: Supplementary file 1 [file appendix_mma.tex]

\begin{table}
    \centering
    \caption{Under the condition that no image information is input to the model, only the text is input for evaluation.}
    \vspace{0.3em}
    \setlength{\tabcolsep}{3pt}
    
    \resizebox{\textwidth}{!}{%
        \begin{tabular}{lccccccccccccc}
            \specialrule{1.5pt}{0pt}{0pt}
            % \rowcolor[HTML]{EFEFEF}
            % & \multicolumn{1}{c|}{Char-Level} & \multicolumn{6}{c|}{Phrase-Level} & \multicolumn{5}{c|}{Sentence-Level} & Avg. \\ \cline{2-14}
            \rowcolor[HTML]{EFEFEF}
             Method & Char/Num & Pres. & Color/Tex & Num. & Shape & Stance & Pos. & Abstract. & Concrete. & Expert. & Act. & \multicolumn{1}{c}{Rel.} &  Avg. MA $\uparrow$\\
            \hline
            Random &25 &25 &25 &25 &25 &25 &25 &25 &25 &25 &25 &25 &25\\
            \hline
            \multicolumn{14}{c}{\textit{Closed-source Models}}\\
            \hline
            Gemini-pro-vision\cite{team2023gemini} &42.50 &50.00 &41.67 &25.00 &83.33 &50.00 &45.45 &40.91 &47.62 &45.16 &70.83 &45.45 &48.67\\ 
            GPT4o\cite{gpt4v} &72.50 &68.18 &66.67 &45.83 &87.5 &70.83 &50.00 &68.18 &76.19 &70.97 &83.33 &63.64 &69.00\\ 
            Qwen-VL-max\cite{bai2023qwenvl} &67.50 &72.73 &66.67 &41.67 &79.17 &62.5 &63.64 &77.27 &80.95 &61.29 &79.17 &72.73 &68.33\\
            Claude3-Opus-V\cite{anthropic2024claude} &35.00 &22.73 &12.50 &16.67 &33.33 &16.67 &22.73 &45.45 &33.33 &25.81 &37.50 &40.91 &28.67 \\
            Step-1V\cite{step1v} &60.00 &54.55 &58.33 &20.83 &70.83 &54.17 &31.82 &54.55 &57.14 &45.16 &79.17 &50.00 &53.33 \\
            Glm-4V\cite{du2022glm} &60.00 &54.55 &54.17 &29.17 &58.33 &41.67 &27.27 &72.73 &47.62 &35.48 &70.83 &45.45 &50.00 \\
            \hline
            \multicolumn{14}{c}{\textit{Open-source Models}}\\
            \hline
            LLaVA-RLHF\cite{sun2023aligning} &7.50 &36.36 &33.33 &33.33 &50.00 &16.67 &9.09 &59.09 &38.10 &22.58 &50.00 &31.82 &30.67\\
            LLaVA-1.6-34B\cite{liu2023llava} &75.00 &68.18 &66.67 &41.67 &79.17 &54.17 &72.72 &81.81 &71.42 &64.52 &79.17 &68.18 &68.67 \\
            Bunny-Llama-3-8B-V\cite{he2024efficient} &55.00 &63.64 &54.17 &37.50 &79.17 &62.50 &54.55 &72.73 &85.71 &48.39 &75.00 &50.00 &60.67\\
            Mini-Gemini-HD-34B\cite{li2024mini} &62.50 &63.64 &70.83 &54.17 &79.17 &62.50 &72.73 &86.36 &85.71 &54.84 &19.17 &68.18 &69.00\\
            Phi-3-vision\cite{abdin2024phi3} &62.50 &59.09 &58.33 &37.50 &70.83 &33.33 &31.82 &54.55 &66.67 &41.94 &58.33 &50.00 &52.33\\
            MiniCPM-Llama3-V\cite{viscpm} &37.5 &45.45 &50.00 &16.67 &41.67 &37.5 &36.36 &68.18 &33.33 &29.03 &41.67 &54.55 &40.33\\
            InternVL-Chat-V1-5\cite{chen2024far} &62.5 &59.09 &66.67 &41.67 &66.67 &41.67 &54.55 &63.64 &66.67 &45.16 &79.17 &72.73 &59.67\\
            Yi-VL-34B\cite{ai2024yi} &52.50 &63.64 &70.83 &41.67 &75.00 &37.50 &59.09 &68.18 &57.14 &48.39 &70.83 &63.64 &58.33 \\
            Deepseek-VL-7B-Chat\cite{lu2024deepseek} &52.50 &54.55 &54.17 &37.5 &62.5 &25.00 &18.18 &54.55 &52.38 &35.48 &75.00 &50.00 &47.67 \\
            Cogvlm2-llama3\cite{wang2023cogvlm} &60.00 &63.64 &54.17 &37.5 &70.83 &33.33 &40.91 &50.00 &85.71 &41.94 &62.50 &50.00 &54.00 \\
            Idefics2-8B\cite{laurençon2024matters} &57.50 &59.09 &54.17 &50.00 &79.17 &41.67 &27.27 &77.27 &76.19 &45.16 &75.00 &40.91 &56.67 \\
            Mplug-owl2-llama2-7B\cite{ye2023mplugowl2} &32.50 &63.64 &58.33 &20.83 &62.50 &37.50 &13.64 &54.55 &47.62 &25.81 &58.33 &31.82 &41.33 \\
            Ours & 50.00 & 59.09 & 54.17 & 25.00 & 83.33 & 50.00 & 54.55 & 63.64 & 66.67 & 51.61 & 79.17 & 54.55 & 57.00 \\
            \specialrule{1.5pt}{0pt}{0pt}
            %             \rowcolor[HTML]{EFEFEF}
            % & \multicolumn{1}{c|}{Char-Level} & \multicolumn{6}{c|}{Phrase-Level} & \multicolumn{5}{c|}{Sentence-Level} & Avg. \\ \cline{2-14}
            \rowcolor[HTML]{EFEFEF}
             Method & Char/Num & Pres. & Color/Tex & Num. & Shape & Stance & Pos. & Abstract. & Concrete. & Expert. & Act. & \multicolumn{1}{c}{Rel.} & Avg. MR $\downarrow$\\
            \hline
            Random &50 &50 &50 &50 &50 &50 &50 &50 &50 &50 &50 &50 &50\\
            \hline
            \multicolumn{14}{c}{\textit{Closed-source Models}}\\
            \hline
            Gemini-pro-vision\cite{team2023gemini} &29.17 &31.25 &41.18 &45.45 &13.04 &40.00 &33.33 &52.63 &44.44 &48.15 &19.05 &23.08 &34.82\\ 
            GPT4o\cite{gpt4v} &9.38 &16.67 &23.81 &26.67 &4.55 &19.05 &38.89 &28.57 &15.79 &24.14 &13.04 &22.22 &19.46\\ 
            Qwen-VL-max\cite{bai2023qwenvl} &22.86 &11.11 &23.81 &28.57 &5.00 &25.00 &30.00 &19.05 &19.05 &29.63 &9.52 &15.79 &20.23\\
            Claude3-Opus-V\cite{anthropic2024claude} &26.32 &50.00 &72.73 &55.56 &50.00 &71.43 &50.00 &37.5 &46.15 &60.00 &43.75 &30.77 &48.50 \\
            Step-1V\cite{step1v} &14.29 &25.00 &26.32 &61.54 &5.56 &40.91 &61.11 &33.33 &33.33 &44.00 &9.52 &21.43 &30.43 \\
            Glm-4V\cite{du2022glm} &27.27 &36.84 &35.00 &56.25 &33.33 &52.38 &53.85 &20.00 &47.37 &57.69 &19.05 &37.50 &38.78 \\
            \hline
            \multicolumn{14}{c}{\textit{Open-source Models}}\\
            \hline
            LLaVA-RLHF\cite{sun2023aligning} &86.36 &50.00 &50.00 &46.67 &40.00 &78.95 &81.82 &38.10 &57.89 &68.18 &29.41 &56.25 &57.01\\
            LLaVA-1.6-34B\cite{liu2023llava} &6.25 &11.76 &20.00 &23.08 &9.52 &35.00 &11.11 &14.28 &25.00 &20.00 &9.52 &16.67 &16.26 \\
            Bunny-Llama-3-8B-V\cite{he2024efficient} &15.38 &22.22 &18.75 &40.00 &5.00 &28.57 &29.41 &23.81 &10.00 &40.00 &10.00 &26.67 &22.22\\
            Mini-Gemini-HD-34B\cite{li2024mini} &21.88 &12.50 &10.53 &7.14 &5.00 &28.57 &15.79 &9.52 &5.26 &32.00 &9.52 &11.76 &15.16\\
            Phi-3-vision\cite{abdin2024phi3} &19.35 &18.75 &26.32 &43.75 &19.05 &55.56 &58.82 &40.00 &22.22 &48.00 &33.33 &31.25 &34.03\\
            MiniCPM-Llama3-V\cite{viscpm} &37.50 &16.67 &33.33 &71.43 &41.18 &47.06 &38.46 &16.67 &41.67 &57.14 &33.33 &25.00 &38.58\\
            InternVL-Chat-V1-5\cite{chen2024far} &21.88 &18.75 &23.81 &37.50 &27.27 &52.38 &29.41 &33.33 &26.32 &44.00 &13.64 &20.00 &28.97\\
            Yi-VL-34B\cite{ai2024yi} &27.59 &22.22 &15.00 &28.57 &10.00 &50.00 &27.78 &16.67 &42.86 &42.31 &22.73 &17.65 &27.39 \\
            Deepseek-VL-7B-Chat\cite{lu2024deepseek} &30.00 &20.00 &27.78 &43.75 &31.82 &71.43 &77.78 &45.45 &47.62 &57.69 &14.29 &38.89 &42.34 \\
            Cogvlm2-llama3\cite{wang2023cogvlm} &22.58 &22.22 &27.78 &30.77 &15.00 &61.90 &35.71 &45.00 &14.29 &51.85 &28.57 &38.89 &33.06 \\
            Idefics2-8B\cite{laurençon2024matters} &23.33 &27.78 &23.53 &20.00 &13.64 &50.00 &40.00 &22.73 &11.11 &41.67 &14.29 &40 &26.72 \\
            Mplug-owl2-llama2-7B\cite{ye2023mplugowl2} &38.10 &17.65 &22.22 &61.54 &25.00 &57.14 &76.92 &40.00 &47.37 &65.22 &26.32 &46.15 &42.86 \\
            Ours & 16.67 & 7.14 & 27.78 & 50.00 & 4.76 & 40.00 & 29.41 & 30.00 & 26.32 & 30.43 & 9.52 & 7.69 & 22.97 \\
            \specialrule{1.5pt}{0pt}{0pt}
        \end{tabular}
    }
    \label{tab:appendix_mma}
\end{table}
